# Supplementary material for: Probing Dark Matter Using Precision Measurements of Stellar Accelerations
Source: arXiv:1812.07578 ancillary file (2019-08-29)
Supplement: Supplementary file 1 [file SM.pdf]

# Probing Dark Matter Using Precision Measurements of Stellar Accelerations: Supplementary Material

Aakash Ravi,<sup>1,2</sup> Nicholas Langellier,<sup>1,2</sup> David F. Phillips,<sup>2</sup>  
Malte Buschmann,<sup>3</sup> Benjamin R. Safdi,<sup>3</sup> and Ronald L. Walsworth<sup>1,2,\*</sup>

<sup>1</sup>*Department of Physics, Harvard University, Cambridge, MA 02138, USA*

<sup>2</sup>*Harvard-Smithsonian Center for Astrophysics, 60 Garden St., Cambridge, MA 02138, USA*

<sup>3</sup>*Leinweber Center for Theoretical Physics, Department of Physics,  
University of Michigan, Ann Arbor, Michigan 48109, USA*

(Dated: December 23, 2018)

## GENERATION OF SYNTHETIC RV TIME SERIES

The observing schedule  $\{t_i\}$  is generated for a total measurement campaign of 10 years, with observing blocks lasting 60 days (to average over stellar rotations), occurring at 1-year intervals. Within the observing blocks, we assume that, for a given target, single exposures are taken every night, and that 1/3 of the nights (generated randomly) are discarded due to the presence of clouds.

We restrict ourselves to solar-type stars (mass range  $0.7 - 1.3M_\odot$ ) so that we may apply well-known models developed for such stars. Taking the simplest possible assumption, we assume the primary star masses  $M_p$  to be uniformly distributed within this range.

Each stellar system is given a random inclination angle  $i$  uniformly distributed between 0 and  $\pi$ , as we are not aware of any anisotropy in this distribution. All bodies orbiting the star are assumed to lie in a single plane inclined at this angle. The inclinations are used to project the RVs along the line of sight. Orbital eccentricities are ignored for simplicity.

First, we will consider the largest Doppler shift contribution: stellar companions. According to stellar multiplicity statistics for solar-type stars [1], 56% of the systems are single, 33% are binary, 8% are triple, and 3% are quadruple and higher. In practice, we truncate the distribution at quadruples for simplicity, i.e., 3% of the stars are given three companions. If a star has a companion, we generate a mass  $M_s$  and period  $T_s$  for this secondary object. The mass may be generated from a mass ratio  $q = M_s/M_p$ ,  $0 \leq q \leq 1$ . The mass ratio follows a power-law distribution [2],  $\sim q^{0.3}$ . Similarly, the period of stellar companions follows a lognormal distribution [1] with mean  $\mu_{\log_{10}(T/\text{days})} = 5.03$  and standard deviation  $\sigma_{\log_{10}(T/\text{days})} = 2.28$ . Using Kepler's third law, we can compute the semimajor axis of the secondary as  $a_s = \sqrt[3]{GM_p T_s^2 / (4\pi^2)}$ , where  $M_p$  is the mass of the primary star. Once we have these orbital parameters, we can sum the radial velocity (RV) contributions of stellar companions for each primary star as

$$v_{\text{comp}}(t) = \sum_k \frac{2\pi}{T_k} q_k a_k \sin(2\pi t/T_k + \phi_k) \sin i, \quad (1)$$

where  $T_k$  is the period of the  $k^{\text{th}}$  stellar companion in the stellar system. Similarly,  $q_k$ ,  $a_k$  and  $\phi_k$  are, respectively,

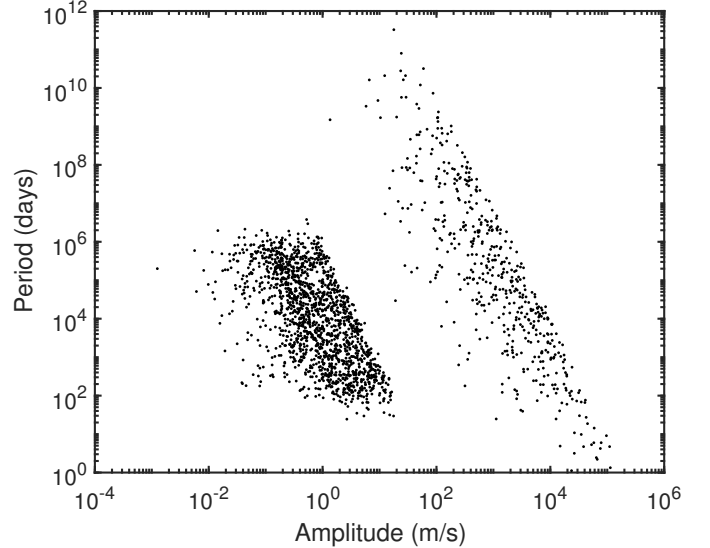

Figure 1. Distribution of periods and semi-amplitudes (weighted by inclination factor  $\sin i$ ) in our synthesized dataset of  $10^3$  primary stars. The group on the left is the set of planets while the group on the right is the set of stellar companions.

the mass ratio, the semimajor axis and orbital phase offset (uniformly distributed between 0 and  $2\pi$ ) for that companion.

Next, we consider the effect of planets in a very similar manner. Statistics from microlensing observations indicate that each Milky Way star hosts, on average, 1.6 planets [3]. We then assign stars  $n$  planets, where  $n$  is a Poisson random variable with mean 1.6, i.e.,  $n \sim \text{Pois}(\bar{n} = 1.6)$ . If a given primary star has any planets, then for each planet, we generate a semimajor axis  $a_{\text{pl}}$  and mass  $M_{\text{pl}}$ . We assume  $\ln a_{\text{pl}}$  is uniformly distributed between 0.4 AU (inner cutoff) and 120 AU (the size of our solar system) as per Ref. [4]. We smooth the edges of this log-uniform distribution appropriately to prevent hard cutoffs. From this information, we can calculate the period using Kepler's third law  $T_{\text{pl}} = \sqrt{4\pi^2 a_{\text{pl}}^3 / (GM_p)}$ . We then compute the planet mass using the statistics for planet radii [5] and use the well-known planetary mass-radius relations [6] to convert radii to masses. We assume the planet radius  $R_{\text{pl}}$  is power-law distributed as  $\sim R_{\text{pl}}^{-2}$  and draw numbers between  $4R_\oplus$  and  $30R_\oplus$  (cutoffs), where  $R_\oplus$  is the radius of the Earth. Once we have both the semimajor axis and mass of the planet, we can sum the RV contributions of the

planets for each primary star as for stellar companions in Eq. (1) to obtain  $v_{\text{plan}}$ . The only difference is that  $q$  in the case of planets is defined as  $M_{\text{pl}}/M_p$ . Together, we refer to  $v_{\text{comp}}$  and  $v_{\text{plan}}$  as Keplerian terms as they are associated with orbiting bodies. Figure 1 shows the distribution of period versus semi-amplitude for the orbiting bodies in our synthesized dataset.

Finally, we include the effects of stellar magnetic activity (henceforth referred to as stellar noise). For a given primary star, the stellar noise contribution is taken to be distributed as a multivariate normal, i.e.,  $v_{\text{noise}}(t) \sim \mathcal{N}(\boldsymbol{\mu}, \mathbf{K})$ . The noise is taken to have zero mean (i.e.,  $\boldsymbol{\mu} = \mathbf{0}$ ) and covariance given by the kernel  $\mathbf{K}$ . The matrix  $\mathbf{K}$  in turn may be expressed as the sum of two parts  $\mathbf{K}_{\text{WN}} + \mathbf{K}_{\text{QP}}$ , a white noise component and a quasiperiodic component. The white noise component, which models the instrumental noise (same for all stars), is given as  $K_{\text{WN}}(t_i, t_j) = \sigma_{\text{WN}}^2 \delta(t_i, t_j)$ , where  $\sigma_{\text{WN}}^2$  is the white noise variance and  $\delta$  is a Kronecker delta. The elements of the quasiperiodic component are given as [7]

$$K_{\text{QP}}(t_i, t_j) = h^2 \exp \left( -\frac{\sin^2 [\pi (t_i - t_j) / T_r]}{2w^2} - \frac{(t_i - t_j)^2}{\lambda^2} \right) \quad (2)$$

where  $h$  is scale of the magnetic activity (in RV units),  $T_r$  is the rotation period of the star,  $w$  is a dimensionless “roughness” parameter and  $\lambda$  is the (stellar) spot lifetime. In our simulations, we take  $\sigma_{\text{WN}} = 0.1$  or  $0.6$  m/s (depending on the scenario),  $h \sim U(0.5, 2.5)$  m/s,  $T_r \sim U(14, 35)$  days,  $w \sim U(0.4, 0.6)$ , and  $\lambda \sim U(20, 30)$  days.  $U(a, b)$  denotes a uniform distribution between  $a$  and  $b$ . In the cases distributions are given, the parameters are drawn from these distributions for each star. The presence of stellar magnetic cycles further causes modulation of  $\boldsymbol{\mu}, \mathbf{K}$  over the cycle period [8] and is straightforward to include in the simulation but is ignored here for simplicity.

## TIME SERIES ANALYSIS USING GAUSSIAN PROCESSES

In order to test the feasibility of a stellar acceleration survey campaign with present-day technology and analysis techniques, RV time series are generated with correlated noise as described above. In order to model the correlated noise, a Gaussian process (GP) regression is employed [7, 9, 10]. A GP assumes the data are normally distributed with mean  $\boldsymbol{\mu}$  and covariance matrix  $\mathbf{K}$ . This allows for a simultaneous fit of any deterministic physics with a model of the correlated noise.

For this analysis, the mean function models both the stellar acceleration and  $M$  Keplerian signals (stellar companions and planets):

$$\mu(t_i) = \Delta a_r t_i + v_{\text{off}} + \sum_{j=1}^M A_j \sin \left( \frac{2\pi t_i}{T_j} + \phi_j \right), \quad (3)$$

where the relative stellar acceleration is  $\Delta a_r$  and the offset

velocity is  $v_{\text{off}}$ . Each orbiting body is assumed to have zero eccentricity so  $A_j$ ,  $T_j$ , and  $\phi_j$  are the RV amplitude, orbital period, and orbital phase offset for the  $j^{\text{th}}$  orbiting body, respectively. The number of Keplerian signals,  $M$ , is chosen by assuming we would have knowledge of some (but not necessarily all) orbiting bodies for a given star. For our fits, we look at each orbiting body injected into the simulation and include it in Eq. (3) if the RV amplitude is greater than 1 m/s and the orbital period is less than  $10^4$  days. The covariance matrix  $\mathbf{K}$  is populated using the quasiperiodic kernel function given in Eq. (2) with an additive white noise term on the main diagonal:

$$K_{i,j} = K_{\text{QP}}(t_i, t_j) + \sigma_{\text{WN}}^2 \delta(t_i, t_j) \quad (4)$$

The GP model thus contains a total of  $7 + 3M$  fit parameters,

$$\boldsymbol{\theta}_{\text{GP}} = \langle \Delta a_r, v_{\text{off}}, \{A_j\}, \{T_j\}, \{\phi_j\}, h, T_r, w, \lambda, \sigma_{\text{WN}} \rangle \quad (5)$$

with a likelihood function given by

$$\mathcal{L}(\mathbf{v}, \mathbf{t} | \boldsymbol{\theta}_{\text{GP}}) = \frac{1}{\sqrt{|2\pi\mathbf{K}|}} e^{-\frac{1}{2}(\mathbf{v}-\boldsymbol{\mu})^T \mathbf{K}^{-1}(\mathbf{v}-\boldsymbol{\mu})}, \quad (6)$$

where  $\mathbf{v}$  is a vector of the measured RVs at times  $\mathbf{t}$ , and  $\boldsymbol{\mu}$  and  $\mathbf{K}$  are functions of  $\mathbf{t}$  and  $\boldsymbol{\theta}_{\text{GP}}$  as described in Equations (3) and (4). The relative stellar acceleration,  $\Delta a_r$ , is given a Gaussian prior with a mean equal to the injected stellar acceleration signal and a standard deviation of 30 times the mean, i.e.,

$$P(\Delta a_r) \sim \mathcal{N} \left( 1.5 \times 10^{-8} \text{ cm/s}^2, 45 \times 10^{-8} \text{ cm/s}^2 \right). \quad (7)$$

This prior is chosen to include the expected value of the relative stellar acceleration and reasonable deviations about this value while rejecting accelerations from long period orbiting bodies that are degenerate with the stellar acceleration signal on the timescale of a decade. The remaining model parameters are allowed to vary freely.

The maximum a posteriori is taken as the parameter estimate,  $\hat{\boldsymbol{\theta}}_{\text{GP}}$ . Minimization of the negative log posterior yields the desired result:

$$\hat{\boldsymbol{\theta}}_{\text{GP}} = \underset{\boldsymbol{\theta}_{\text{GP}}}{\text{argmin}} [-\ln \mathcal{L}(\mathbf{v}, \mathbf{t} | \boldsymbol{\theta}_{\text{GP}}) - \ln P(\Delta a_r)]. \quad (8)$$

Minimization is performed using the quasi-Newton method of Broyden, Fletcher, Goldfarb, and Shanno [11]. Initial guesses for the model parameters,  $\boldsymbol{\theta}_{\text{GP},0}$ , were chosen assuming we would have knowledge of their true values,  $\boldsymbol{\theta}_{\text{GP}, \text{true}}$ . The values were normally distributed about their true value with a standard deviation of about 3% of the mean, i.e.,

$$P(\boldsymbol{\theta}_{\text{GP},0}) \sim \mathcal{N} \left( \boldsymbol{\theta}_{\text{GP}, \text{true}}, \frac{1}{30} \boldsymbol{\theta}_{\text{GP}, \text{true}} \right). \quad (9)$$

The Python [12] packages NumPy [13], SciPy [14], and George [15] were used for this analysis.

## CONSIDERATIONS FOR OBSERVING TARGETS

When designing the stellar acceleration survey, one consideration is the volume of space needs that to be surveyed to observe about  $10^3$  target Sun-like stars. The local stellar density in the solar neighborhood<sup>1</sup> is  $0.1 \text{ pc}^{-3}$ , and we conservatively assume the same density at  $\sim$  few kpc inward toward the Galactic Center (GC) relative to the Sun. Further, if we assume only approximately 5% of the stars are of spectral type G, we would need an observation box of side length  $\sim 60 \text{ pc} = 200 \text{ ly}$ .

Another important consideration is star visibility. Using Sagittarius A\* as an indicator of the GC and a sky model<sup>2</sup> for the Paranal Observatory in Chile ( $24^\circ 37' 38''\text{S}$   $70^\circ 24' 15''\text{W}$ ), we find that the GC is visible about 8 out of 12 months a year.

Finally, we also consider exposure times for targets. First we compute the apparent magnitude  $m$  of a Sun-like star at distance  $\Delta r$  away from its absolute magnitude  $M = 4.83$ . The apparent magnitude at various distances are: 14.8 (1 kpc away) and 17.2 (3 kpc away). We feed these magnitudes into exposure time calculators for current precision RV spectrographs at 3.6 m telescopes<sup>3</sup> and 10 m telescopes<sup>4</sup>, and appropriately scale by telescope diameters, i.e.,  $t_{\text{exp}} / (D_{\text{next-gen}} / D_{\text{current}})^2$ . With a target signal-to-noise ratio of 100, we get  $t_{\text{exp}} = 12 \text{ min}$  for a target  $\Delta r = 1 \text{ kpc}$  away with a 30-meter telescope, or alternatively for a target  $\Delta r = 3 \text{ kpc}$  away with a 100-meter telescope (e.g., Overwhelmingly Large Telescope [16]). Given an average night of 8 hours, and the visibility issue discussed above (duty cycle 2/3), we calculate that this exposure time would limit the number of observations to  $10^4 / N$  per star per year for a  $N$ -star survey if a single telescope was the only resource for the project. It should be noted that the stellar acceleration change  $\Delta a_r$  increases linearly with distance from the Sun  $\Delta r$ , but the total telescope exposure time grows quadratically with distance. So one wins by doing very precise measurements at shorter range until more advanced telescope technology becomes available. One can also go to intermediate distances and mea-

sure for longer than a decade.

---

\* [rwalsworth@cfa.harvard.edu](mailto:rwalsworth@cfa.harvard.edu)

- [1] D. Raghavan, H. A. McAlister, T. J. Henry, D. W. Latham, G. W. Marcy, B. D. Mason, D. R. Gies, R. J. White, and T. A. ten Brummelaar, *Astrophys. J. Suppl. Ser.* **190**, 1 (2010).
- [2] G. Duchêne and A. Kraus, *Annu. Rev. Astron. Astrophys.* **51**, 269 (2013).
- [3] A. Cassan, D. Kubas, J.-P. Beaulieu, M. Dominik, K. Horne, J. Greenhill, J. Wambsganss, J. Menzies, A. Williams, U. G. Jørgensen, *et al.*, *Nature* **481**, 167 (2012).
- [4] L. Zeng, S. B. Jacobsen, D. D. Sasselov, and A. Vanderburg, (2018), [arXiv:1801.03994](https://arxiv.org/abs/1801.03994).
- [5] L. Zeng, S. B. Jacobsen, D. D. Sasselov, and A. Vanderburg, (2018), [arXiv:1801.03993](https://arxiv.org/abs/1801.03993).
- [6] D. Bashi, R. Helled, S. Zucker, and C. Mordasini, *Astron. Astrophys.* **604**, A83 (2017).
- [7] S. Roberts, M. Osborne, M. Ebdon, S. Reece, N. Gibson, and S. Aigrain, *Philos. Trans. Royal Soc. A* **371**, 20110550 (2013).
- [8] N. Meunier, A.-M. Lagrange, and M. Desort, *Astron. Astrophys.* **519**, A66 (2010).
- [9] C. E. Rasmussen and C. K. I. Williams, *Gaussian Processes for Machine Learning* (MIT Press, 2006).
- [10] R. D. Haywood, A. Collier Cameron, D. Queloz, S. C. C. Barros, M. Deleuil, R. Fares, M. Gillon, A. F. Lanza, C. Lovis, C. Moutou, *et al.*, *Mon. Not. Roy. Astron. Soc.* **443**, 2517 (2014).
- [11] J. Nocedal and S. J. Wright, *Numerical Optimization*, edited by P. Glynn and S. M. Robinson (Springer, 1999) pp. 136–138.
- [12] G. van Rossum, *Python tutorial*, Tech. Rep. CS-R9526 (Centrum voor Wiskunde en Informatica (CWI), Amsterdam, 1995).
- [13] T. Oliphant, “NumPy: A guide to NumPy,” USA: Trelgol Publishing (2006).
- [14] E. Jones, T. Oliphant, P. Peterson, *et al.*, “SciPy: Open source scientific tools for Python,” (2001).
- [15] S. Ambikasaran, D. Foreman-Mackey, L. Greengard, D. W. Hogg, and M. O’Neil, [arXiv:1403.6015](https://arxiv.org/abs/1403.6015).
- [16] R. Gilmozzi, B. Delabre, P. Dierickx, N. N. Hubin, F. Koch, G. J. Monnet, M. Quattri, F. J. Rigaut, and R. N. Wilson, *Proc. SPIE* **3352**, 778 (1998).

---

<sup>1</sup> RECONS Census Of Objects Nearer Than 10 Parsecs

<sup>2</sup> SkyCalc Sky Model Calculator

<sup>3</sup> HARPS Exposure Time Calculator

<sup>4</sup> HIRES Exposure Time Calculator
